# Supplementary material for: Understanding VSIDS Branching Heuristics in Conflict-Driven Clause-Learning SAT Solvers
Source: arXiv:1506.08905 source file (2015-09-14)
Supplement: Supplementary file 1 [file appendix.tex]

\section{\appendixname}

For the purposes of the discussion below, consider a dynamically
evolving TVIG G of variables/clauses of a Boolean formula F input to a
SAT solver. The graph G evolves as the solver learns new clauses and
adds it to the learnt clause database. Further assume that G is
modified only through addition of nodes/edges (correspondingly,
variables/clauses in F), without any deletions or morphing of
nodes/edges (correspondingly, no clause deletion or
in-processing). Further assume that the \cvsids ranking is initialized
to the ranking produced by the TDC measure over the TVIG
of the input formula F. Under these assumptions, the \cvsids ranking
of F and learnt clauses, at any point during the solving process, will
exactly match the TDC rankings of the nodes of the dynamically
evolving TVIG G of F and learnt clauses. We prove this formally below.

For the theorem below, we use the following definitions, notations and
conventions. The goal is to abstract away those inner-workings of CDCL
SAT solvers that are irrelevant here.

\vs \vs
\noindent{\bf 8.1 Definitions}
\begin{description}

\item[Ranking:] of variables (resp. nodes) in a Boolean formula F
  (resp. TVIG G): Consider a set of pairs, where the first element is
  a variable in F (resp. corresponding node in G), and the second
  element is a real number. A ranking R(F) over F (resp. R(G) over G)
  is a decreasing order over such pairs based on the decreasing order
  over the real numbers in these pairs. We say two rankings $R_1$ and
  $R_2$ match (or are equal), written as $R_1 = R_2$, if every
  $i^{th}$ element of $R_1$ and $R_2$ are pairwise equal.

\vs \vs
\item[Linearly-ordered Family of TVIG graphs:] We say $G = {g_0, g_1,
  g_2,...}$ represent a linearly-ordered family of TVIG for a
  corresponding family $F = {f_0,f_1,f_2,...}$ of Boolean formulas, if
  the following conditions hold: 
\begin{itemize}
  \item $g_i$ is the TVIG of $f_i$
  \item $f_i$ (resp. $g_i$) is obtained from $f_{i-1}$
    (resp. $g_{i-1}$) only by adding a single clause $c$ (resp. edges
    among the nodes corresponding to $c$ in $g_{i-1}$), without any
    other modifications/deletions to existing clauses in
    $f_{i-1}$. 
\item For all $i$, $f_i$ share the same variables.
\end{itemize}
 
\vs \vs
\item[The \cvsids Function:] We need a precise treatment of \cvsids
  heuristic in order to prove the theorem. We say that the \cvsids
  function takes as input a formula $f_i$ and the ranking of the
  variables over the formula $f_{i-1}$. Every variable in $f_i$ get
  assigned the ranking of the corresponding variable in
  $f_{i-1}$. Additionally, \cvsids bumps by 1 the ranks of the
  variables of the clause added to $f_{i-1}$ to obtain $f_i$, and
  multiplicatively decays the ranks of all variables. It then orders
  the ranks and outputs it.

\end{description}

\noindent{\bf 8.2 The Proof of \cvsids Centrality Theorem}

\begin{theorem}
Let $R_{\cvsids}(f_i)$ denote the ranking produced by the \cvsids
function over the formula $f_i$. Similarly, let $R_{TDC}(g_i)$ denote
the ranking produced by the TDC measure over the graph $g_i$. If
$R_{\cvsids}(f_{i}) = R_{TDC}(g_{i})$ then for all $j>i$
$R_{\cvsids}(f_j) = R_{TDC}(g_j)$.
\end{theorem}

\begin{proof} (by Induction)

\vs \vs
\noindent{We prove the theorem by by induction on $i$.}

\vs \vs
\noindent{\bf Base case:} We note that the variant of \cvsids we
consider initializes the ranking (i.e., $i=0$) of variables in $f_0$
with the TDC ranking over $g_0$.

\vs \vs
\noindent{\bf Inductive Hypothesis:} Assume that $R_{\cvsids}(f_{i}) =
R_{TDC}(g_{i})$.

\vs \vs
\noindent{\bf Inductive Step:} 

\vs Let $c$ be a clause added to $f_{i}$ to obtain
$f_{i+1}$. Correspondingly, we add appropriate edges to the TVIG
$g_{i}$ to obtain $g_{i+1}$. Let $v$ be a variable in $c$, and the
corresponding node in $g_i$ is also denoted as $v$. In the TVIG
$g_{i+1}$, the node $v$ gains $|c|-1$ more edges over the
corresponding node $v$ in $g_{i}$, each of weight
$\frac{1}{|c|-1}$. This adds $1$ to the TDC of
$v$. Therefore the TDC of $v$ is increased by
$1$. Likewise, \cvsids bumps the activity of $v$ (and other variables
in the added clause) by $1$.  Hence \cvsids and TDC
increases activity/centrality by the same amount on each new learnt
clause.

\cvsids then decays the activities by multiplying by a constant decay
factor $\alpha$, where $0<\alpha<1$. Likewise, the TVIG decays the
weights of the edges by the same decay factor. Therefore the equality
between the activity score of variables and their TDC is
maintained.
\end{proof}

This theorem analytically explains the correlation between \cvsids and
TDC. Although SAT solvers typically set the
initial activites of variables to zero, we seed them to be the same as
the TDC in this Section. This enables us to prove
the theorem.

We do not consider clause deletion and in-processing while proving the
above theorem. The reason is that these two operations modify the TVIG
of the original+learnt clauses, thus introducing discrepancies between
\cvsids and TDC that are difficult to account for analytically. Having
said that, in the paper we experimentally showed that
\cvsids and TDC are highly correlated even in the presence of clause
deletion and in-processing.

In the following we empirically verify the theorem, and thus show
that, under our assumptions, the theorem is relevant in practice.

\vs \vs
\noindent{\bf 8.3 Experiment: \cvsids Centrality Theorem}
\vs \vs

\begin{table}[H]
\centering
\begin{tabular}{ | l c | }
\hline
& \quad\cvsids vs TDC\quad \\ 
\hline
Mean top-10     & 0.977 \\      
%Mean percentile & 0.999 \\
Mean Pearson    & 0.998 \\
\hline
\end{tabular}
\vs \vs
\caption{Results of \cvsids Centrality Theorem experiment.}
\end{table}

In this experiment, clause deletion and in-processing are switched off and
the initial \cvsids activity scores are initialized with the initial TDC of
the original clauses. The idea is to control the experiment to replicate the
conditions of the \cvsids Centrality Theorem as closely as possible to
empircally reinforce the theorem. The data shows an almost perfect Pearson
correlation of 0.998. Also 0.977 of the top-ranked \cvsids variables are also
highly ranked in TDC. The reason the metrics are not equal to 1.000
is likely due to the loss of precision from working with very large floating
point numbers. The Sat4j implementation of VSIDS is based off the scheme
introduced by MiniSAT, coined by Biere as EVSIDS~\cite{armin2008}. Instead of
decrementing the activity scores of each variable on each decay, Sat4j will
multiplicatively increase the bump amount for all future bumps. Once the
activity scores exceed $10^{100}$, all the scores will be scaled down by a
factor of $10^{100}$. Arithmetic on large 64-bit floating point numbers will
lead to a loss of precision.

%% \begin{figure}[h]
%% \begin{center}
%% \includegraphics[width=0.85\textwidth]{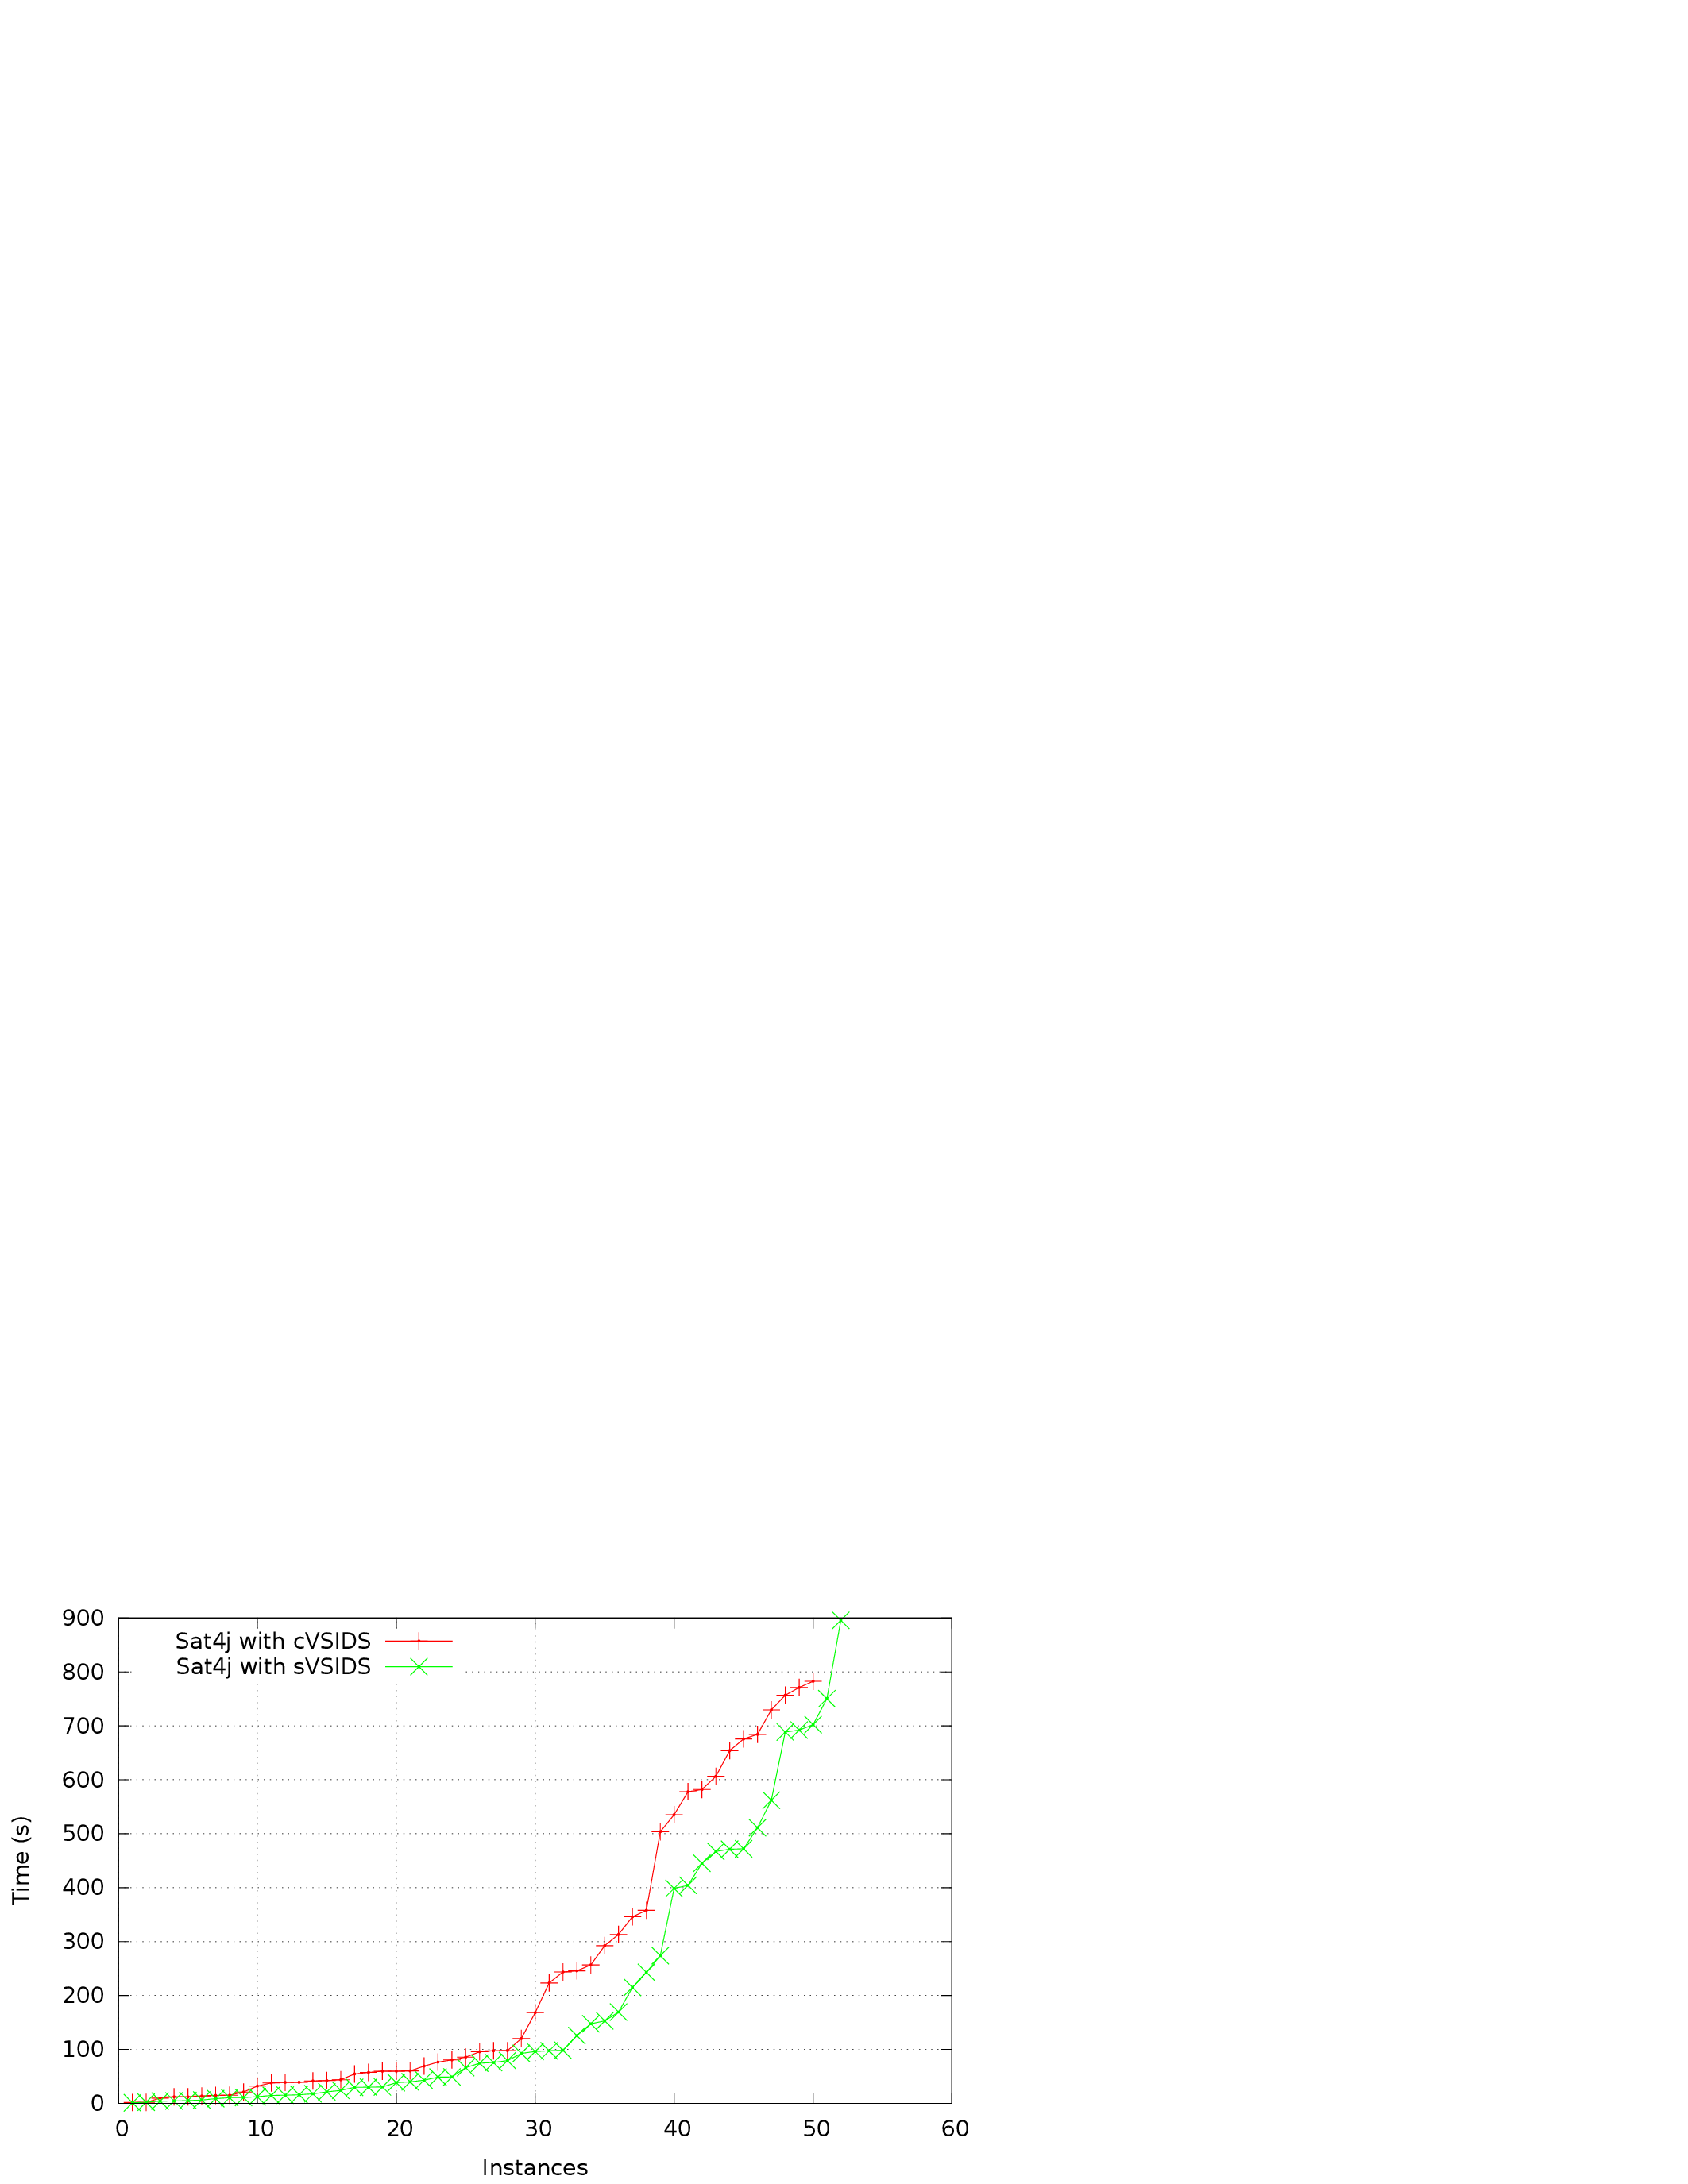}
%% \end{center}
%% \caption{The running times of sVSIDS and cVSIDS for the 100 SAT-Race 2010 benchmarks.}
%% \label{fig:csvsidsvssvsids}
%% \end{figure}
